# Supplementary material for: Tuning Synthetic Semiflexible Networks by Bending Stiffness
Source: arXiv:1610.00909 ancillary file (2016-10-04)
Supplement: Supplementary file 1 [file supplement.pdf]

# Supplemental Material: Tuning Synthetic Semiflexible Networks by Bending Stiffness

Carsten Schuldt,[1,2] Jörg Schnauß,[1,2] Tina Händler,[1,2] Martin Glaser,[1,2] Jessica Lorenz,[2] Tom Golde,[1] Josef A. Käs,[1] and David M. Smith[2]

[1] *Institute of Experimental Physics I, Universität Leipzig, Linnéstraße 5, 04103 Leipzig, Germany*
[2] *Fraunhofer Institute for Cell Therapy and Immunology, Perlickstraße 1, 04103 Leipzig, Germany*

## I MATERIALS & METHODS

### DNA $n$-helix tubes ($n$HT)

Lyophilized oligonucleotides (biomers.net GmbH, Germany) were resuspended in millipore water. Sequences are given in Tab. SI. Concentration was determined by a NanoDrop 1000 (Thermo Fisher Scientific Inc., USA). Final DNA $n$HT samples consisted of the $n-1$ strands $U_1 - U_{n-1}$ and one $T_n$ strand, each at the same monomer concentration. Final buffer conditions were 1xTE (10 mM Tris, 1 mM EDTA, pH 8) and 12.5 mM $MgCl_2$. A thermocycler (TProfessional Standard PCR Thermocycler, Core Life Sciences Inc., USA) was used to hybridize the $n$HTs (randomization and dehybridization for 10 min at 90 °C; complementary base pairing in 20 temperature steps of −0.5 K for 30 min each, starting from 65 °C; quick drop to 20 °C). Hybridized $n$HTs were stored for up to 3 weeks at 4 °C with no detectable degradation. For fluorescence microscopy, labeled $n$HTs were hybridized by substituting $U_1$ with the modified $U_1$-Cy3.

| Name | Sequence |
|---|---|
| U1 | GGCGATTAGG-ACGCTAAGCCA-CCTTTAGATCC-TGTATCTGGT |
| U1-Cy3 | Cy3-TTGGCGATTAGG-... |
| | ...-ACGCTAAGCCA-CCTTTAGATCC-TGTATCTGGT |
| U2 | GGATCTAAAGG-ACCAGATACA-CCACTCTTCC-TGACATCTTGT |
| U3 | GGAAGAGTGG-ACAAGATGTCA-CCGTGAGAACC-TGCAATGCGT |
| U4 | GGTTCTCACGG-ACGCATTGCA-CCGCACGACC-TGTTCGACAGT |
| U5 | GGTCGTGCGG-ACTGTCGAACA-CCAACGATGCC-TGATAGAAGT |
| U6 | GGCATCGTTGG-ACTTCTATCA-ATGCACCTCC-AGCTTTGAATG |
| U7 | GGAGGTGCAT-CATTCAAAGCT-AACGGTAACTA-TGACTTGGGA |
| U8 | TAGTTACCGTT-TCCCAAGTCA-AACACTAGAC-ACATGCTCCTA |
| U9 | GTCTAGTGTT-TAGGAGCATGT-CGAGACTACAC-CCTTGCCACC |
| U10 | TGTAGTCTCGG-GTGGCAAGGG-TACTACCGCT-CCATTAAGAAT |
| U11 | AGCGGTAGTA-ATTCTTAATGG-ATCCGTCTATC-TACACTATCA |
| U12 | ATAGACGGATT-GATAGTGTAG-AGACGAAATC-AGCAGAACTAA |
| U13 | GATTTCGTCT-TTAGTTCTGCT-CTGCGAAGTAA-TCAGCCGAGC |
| T4 | GGTTCTCACGG-ACGCATTGCA-CCTAATCGCC-TGGCTTAGCGT |
| T5 | GGTCGTGCGG-ACTGTCGAACA-CCTAATCGCC-TGGCTTAGCGT |
| T6 | GGCATCGTTGG-ACTTCTATCA-CCTAATCGCC-TGGCTTAGCGT |
| T8 | TAGTTACCGTT-TCCCAAGTCA-CCTAATCGCC-TGGCTTAGCGT |
| T9 | GTCTAGTGTT-TAGGAGCATGT-CCTAATCGCC-TGGCTTAGCGT |
| T10 | GTGTAGTCTCG-GGTGGCAAGG-CCTAATCGCC-TGGCTTAGCGT |
| T14 | TTACTTCGCAG-GCTCGGCTGA-CCTAATCGCC-TGGCTTAGCGT |

Table SI. DNA sequences for the hybridization of all used $n$HTs.

### Actin

G-actin was prepared from rabbit muscle as described previously [1]. Actin was labeled fluorescently by addition of Phalloidin-TRITC (Sigma-Aldrich, USA). Actin polymerization was initiated by the addition of 10 times concentrated F-Buffer (1 M KCl, 10 mM $MgCl_2$, 2 mM ATP, 10 mM DTT, 20 mM phosphate buffer, pH 7.5).

### Atomic Force Microscopy

AFM images were acquired with a NanoWizard 3 (JPK Instruments, Germany). Pre-hybridized 8HT were deposited on freshly cleaved mica. After a settling time of 10 min samples were spun at 6000 rpm in short intervals to minimize alignment of attached $n$HTs. Images were recorded in tapping mode in air at room temperature at a scan rate of 1 line/s. Gold-coated ACTA tips (ACTA-10, AppNano) were used with a spring constant $\sim 54\,\mathrm{N\,m^{-1}}$ and a resonance frequency $\sim 300\,\mathrm{kHz}$.

### Shear rheology

Prior to loading 175 µl of sample to the dynamic shear rheometer (ARES, TA Instruments, USA), the surfactant Triton X-100 (Sigma-Aldrich Co., USA) was added to a final concentration of 0.1 mM. A cone-plate geometry was used (diameter 25 mm,0.04 rad) and the sample was equilibrated for 2 h at 25 °C. The sample chamber was equipped with a water bath and sealed with a cap to suppress evaporation. Measurements were performed at 25 °C and involved the following sequence: (i) short frequency sweep ($\gamma = 5\,\%$, f = 0.01 Hz to 30 Hz, 5 data points per decade), (ii) long frequency sweep ($\gamma = 5\,\%$, f = 0.001 Hz to 30 Hz, 21 data points per decade), (iii) short frequency sweep, (iv) strain sweep ($f = 1$ Hz, $\gamma$ = 0.0125 % to 100 %, 20 data points per decade), (v) a short frequency and (vi) a strain sweep. Raw data was binned (bin size = 3 data points) for Fig. 2(c) & 4(a) of the main text. In Fig. 3(a) and (c) of the main text, $G_0 = G'(f = 1\,\mathrm{Hz}, \gamma = 5\,\%)$ was smoothed with a Gaussian kernel (standard deviation = 2 data points, width =

7 data points) for each measurement and averaged over all measurements (ii) to (iv) and for up to 3 samples per condition.

## II PERSISTENCE LENGTH

Persistence lengths ($l_\mathrm{p}$) of DNA $n$HTs were measured by analyzing the conformations of adsorbed filaments. Here, we found perfect agreement with previous data derived from freely-fluctuating filaments [2].

Fluorescently labeled $n$HTs were hybridized at 2 µM to 8 µM per oligonucleotide. 14HTs for single filament microscopy were hybridized longer (randomization and dehybridization for 10 min at 90 °C; complementary base pairing in 50 temperature steps of −0.2 K for 99 min each, starting from 65 °C; quick drop to 20 °C). Samples were step-wise diluted to 10 nM for observation. Subsequently, 10 µl of the sample solution were placed between two glass slides. This sample chamber was sealed with vacuum grease and nail polish to prevent evaporation. After a settling time of 1 to 20 hours, images of single, adsorbed filaments were recorded via an epi-fluorescence microscope (Leica DM-IRB, 100x objective, NA 1.35) with an attached CCD camera (Andor, iXon DV887). Filament backbones were determined by the ImageJ plugin JFilament (http://imagej.nih.gov/ij/) [3]. More than 100 different filaments were analyzed for each type of $n$HT and full sets of these contours are shown in Fig. S1. With a self-written Matlab program, the 2D tangent-tangent correlation

$$\langle \vec{t}(s) \cdot \vec{t}(s+\Delta s) \rangle = \langle \cos(\theta(\Delta s)) \rangle = \exp\left[-\Delta s / 2 l_\mathrm{p}\right] \quad \text{(S1)}$$

of tangent vectors separated by the arc length shift $\Delta s$ was calculated for all $n$HTs and fitted with equation S1 to obtain $l_\mathrm{p}$. A bootstrap analysis was performed to estimate the error of $l_\mathrm{p}$. For each type of $n$HT with $m$ different filaments, 5000 subsets of $m$ filaments were randomly drawn (with replacement) from the full set of $m$ contours and the tangent-tangent correlation analysis was performed. The mean of $l_\mathrm{p}$ for each of the 5000 subsets was determined as the $l_\mathrm{p}$ for the according $n$HT type. The standard deviation serves as an estimator for the error of $l_\mathrm{p}$. An overview of these values is given in Tab. SII. Schiffels et al. measured $l_\mathrm{p}$ values by observing fluctuations of filaments in two dimensions while immersed in solution [2]. Results of both approaches compare well as illustrated in Fig. S2.

Schiffels et al. argued that it was not possible to measure fixed filaments due to flow from pipetting or adhesion problems. In rare cases where we observed an apparent flow pattern or flow-induced alignment, we omitted the sample. To ensure that filaments were properly equilibrated on the glass surface, we performed a kurtosis analysis of the angle distribution between the tangent

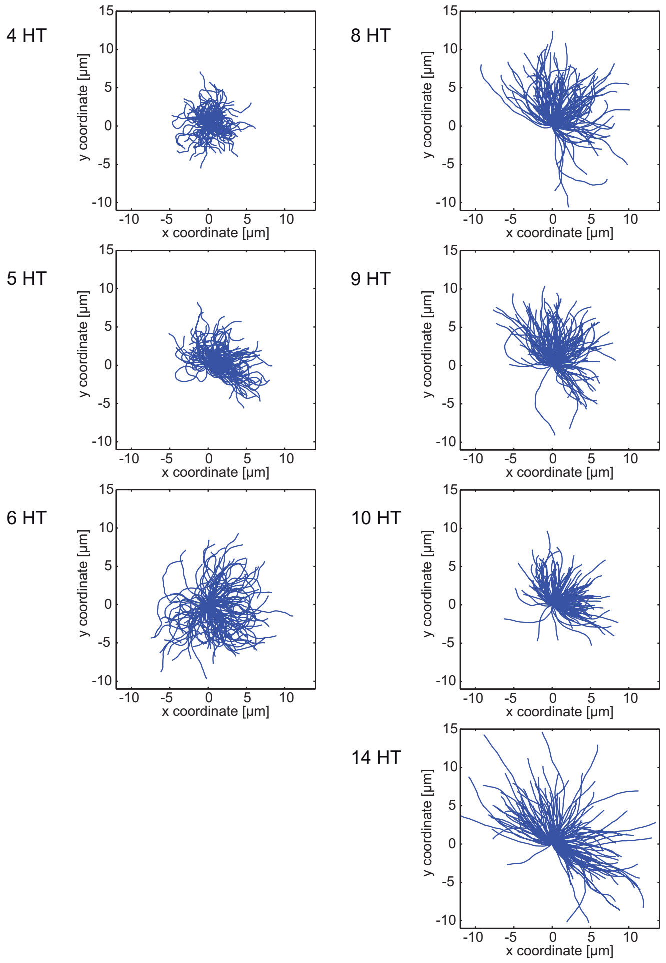


Figure S1. Contours of all $n$HTs. A full set of contours is shown for each type of $n$HT which was evaluated to obtain $l_\mathrm{p}$. All contours start at the origin.

| $n$HT | $l_\mathrm{p}$[µm] | number of filaments |
|---|---|---|
| 4HT | $1.2 \pm 0.1$ | 113 |
| 5HT | $2.0 \pm 0.2$ | 122 |
| 6HT | $3.2 \pm 0.3$ | 120 |
| 8HT | $8.9 \pm 0.9$ | 121 |
| 9HT | $9.7 \pm 1.6$ | 134 |
| 10HT | $12.7 \pm 1.2$ | 144 |
| 14HT | $26.2 \pm 4.8$ | 134 |

Table SII. Persistence length values of all studied $n$HT types.

vectors [4, 5]. The angle's probability distribution function in 2D is given by

$$P\left(\theta\left(\Delta s\right)\right) = \sqrt{\frac{l_\mathrm{p}}{2\pi\Delta s}} \exp\left[-\frac{l_\mathrm{p}\theta^2}{2\Delta s}\right]. \quad \text{(S2)}$$

Only in the case that the distribution function was normal, filaments were considered to be equilibrated in 2D and equation S1 was applicable. The normality can be tested by calculating the kurtosis of $P\left(\theta\left(\Delta s\right)\right)$ via

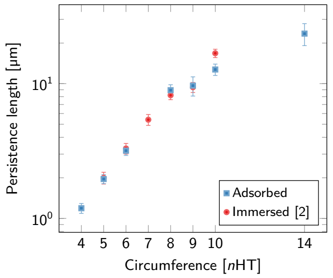


Figure S2. Persistence lengths of different $n$HTs determined from different methods. $l_\mathrm{p}$ was previously derived from freely-fluctuating, immersed $n$HTs [2]. Here, this data was confirmed and extended by studying adsorbed $n$HTs.

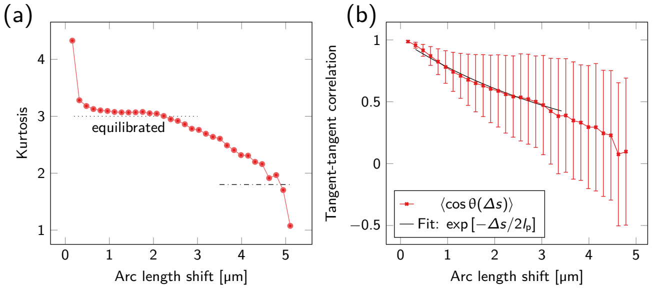


Figure S3. Kurtosis analysis. (a) Kurtosis analysis for angle distribution function of the full set of contours of 5HTs is shown. Red circles depict the data, the dotted line illustrates the theoretical value of 3 for a perfectly normal distribution, and the dash-dotted line at the value 1.8 emphasizes the region where angles are fully uncorrelated. (b) Tangent angle correlation is displayed for the example of the full set of contours of 5HTs. Red crosses show the data and their standard deviation from averaging over all filaments. The black line illustrates a fit with equation S1 with the parameter $l_\mathrm{p}$ yielding 1.9 µm. The fit was restricted to the indicated region, given by kurtosis analysis.

$\left\langle \theta^4(\Delta s)\right\rangle / \left\langle \theta^2(\Delta s)\right\rangle^2$ [4, 5]. A kurtosis value of 3 indicates a normal distribution, whereas 1.8 marks a completely random distribution. For each bootstrapping subset, the kurtosis was analyzed and only arc length values $s$ with a kurtosis between 3.5 and 2.5 were used for subsequent $l_\mathrm{p}$ calculation. An exemplary kurtosis analysis is depicted in Fig. S3. Thus, only equilibrated sections of the $n$HTs were employed for evaluation. The close match with the $l_\mathrm{p}$ derived alternatively [2] confirms this approach (cf. Fig. S2).

## III REPTATION AND MESH SIZE

Reptation experiments confirmed the entangled nature of the $n$HT networks and were used to deduce the mesh size of the according $n$HT type and actin networks. A sample size of 15 µl was prepared with the sample chamber technique described above and imaged accordingly. Additionally, glass slides were passivated with Sigmacote (Sigma-Aldrich, USA) to prevent the filaments from sticking to the surface. Pre-hybridized unlabeled and labeled $n$HTs were mixed at a ratio of 4000:1 and equilibrated overnight at 4 °C. For actin mesh sizes, monomeric unlabeled actin was mixed with pre-polymerized, labeled F-actin at a molar ratio of approximately 2000:1. Actin background network assembly was triggered by addition of 10x F-Buffer. Reptation was observed after one hour of equilibration at a capture frame rate of 10 Hz.

To evaluate mesh sizes, we used the reported correlation [6] of the reptation tube width $a$ with the mesh size $\xi$ and the persistence length $l_\mathrm{p}$

$$a \sim \xi^{6/5} l_\mathrm{p}^{-1/5}. \qquad \text{(S3)}$$

More recently, explicit formulae to extract the mesh size from reptation tube measurements were developed [7, 8]. Even a length correction term was introduced, which accounts for the fact that filaments with a longer contour length $l_\mathrm{c}$ "feel" more of the surrounding network [7]. These approaches lead to the relation

$$a \sim 0.31\, \xi^{6/5} l_\mathrm{p}^{-1/5} + 0.56\, \xi^2 l_\mathrm{c}^{-1}. \qquad \text{(S4)}$$

With equation S4, the mesh size can be implicitly calculated if the persistence length, the contour length, and the tube width for a reptating test filament are known. To obtain the tube width, we summed up all pictures of a reptating filament taken for one minute. This summed picture was subsequently evaluated with JFilament to determine a mean tube backbone (Fig. S4(a)).

Additionally, all individual filament backbones were extracted from the picture time series. Using a self-written Matlab code, all individual contours were plotted with the tube backbone (Fig. S4(b)). From these individual contours, the filament's contour length $l_\mathrm{c}$ was acquired as the mean contour length during the first ten seconds of the measurement. Perpendicular tube profile lines at the backbone points were drawn to determine intersection points between all individual filament contours and the profile lines. For each profile, a kernel density estimation from the intersection points was calculated while the bandwidth of the kernel-smoothing window was set to the width of an individual filament (Fig. S4(c)). For the 8HT [9] this width is 7.6 nm, while the respective value for actin filaments is 8.0 nm [10]. Subsequently, the kernel density of each profile line was fitted by a Gaussian. The tube width at every single tube backbone point is defined as twice the standard deviation of the corresponding Gaussian. Single tube widths along the tube backbone were averaged in the middle region of the tube to determine the final reptation tube width a (Fig. S4(d)). Tube widths and contour lengths of single test filaments were measured for a range of concentrations and the corresponding mesh size was calculated. The results

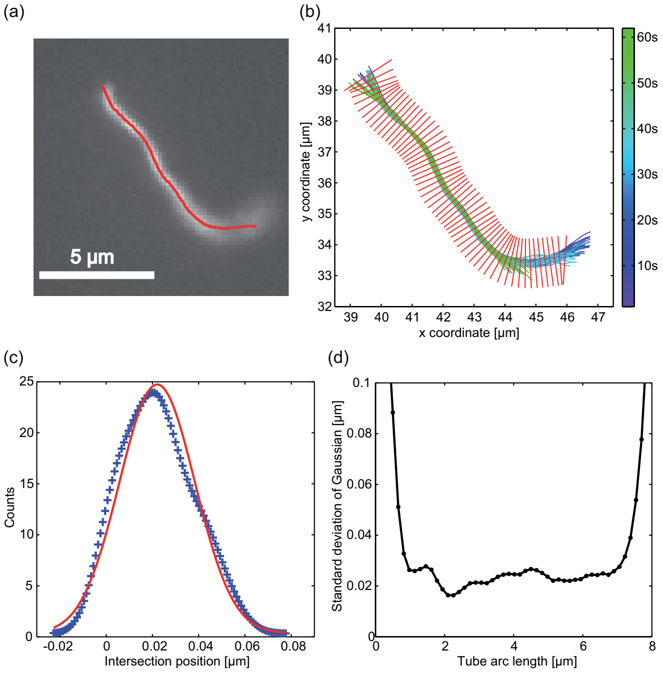


Figure S4. Steps of reptation tube width determination (example 8HT at 20 µM). (a) Sum of all reptation pictures with tube backbone overlay (red). (b) Overlay of all individual filament configurations and perpendicular profile lines (red). Contour color coding indicates the time course. (c) Kernel density estimate (blue crosses) of intersection points between individual configurations and one profile line and according Gaussian fit (red line) are shown. (d) Plot of standard deviations obtained from Gaussian fits versus tube arc length are displayed. Standard deviation is averaged in the middle tube region (from 1 µm to 7 µm in the depicted case). The resulting mean standard deviation is multiplied by 2 to obtain the tube width.

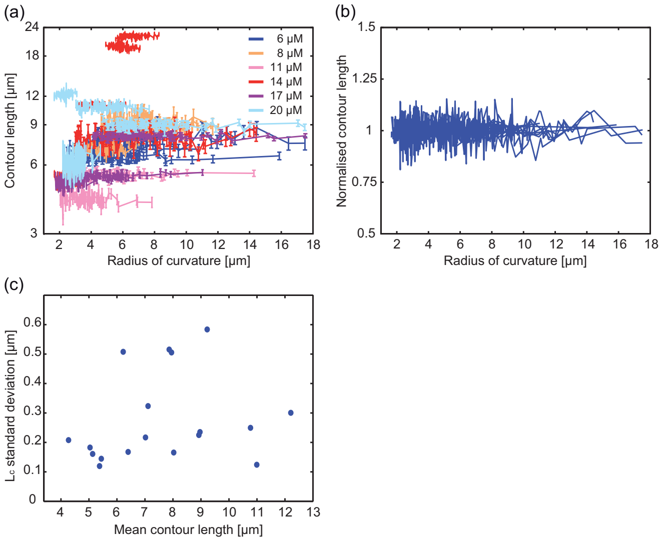


Figure S5. Inextensibility of 8HTs is demonstrated by (a) the plot of contour length vs. radius of curvature for reptating 8HTs in networks of different concentrations (see legend). (b) Normalized contour length curves all collapse onto a single, constant master curve. (c) The standard deviation does not correlate with contour length. Hence, the distribution width is governed by additive systematic detection error.

show a decrease in mesh size with increasing concentration (see Fig. 4(b) in the main text).

## IV INEXTENSIBILITY OF DNA TUBES

Semiflexible polymers are described by the inextensible worm-like chain, where inextensibility is set by the condition

$$\left|\frac{\partial \vec{r}}{\partial s}\right| = \left|\vec{t}\right| = 1. \qquad \text{(S5)}$$

We confirm this prerequisite by studying the contour length $l_\mathrm{c}$, its correlation with the radius of curvature, and the standard deviation $\sigma\left(l_\mathrm{c}\right)$ of reptating 8HTs. Thermally excited stretching modes should reflect in extended contour lengths in highly curved configurations. Correspondingly, the distribution width $\sigma\left(l_\mathrm{c}\right)$ of acquired contour lengths should increase at least with $\sqrt{l_\mathrm{c}}$ for increasing contour length for extensible filaments. Systematic detection errors would reflect in a constant $\sigma\left(l_\mathrm{c}\right)$. Reptation videos were acquired and processed as for mesh size measurements. Tracked contours of the first 10 s of measurement time, i.e. 100 contours, were analyzed with a self-written Matlab program. For each frame, the contour was approximated with a B-Spline representing $\vec{r}(s)$. The mean radius of curvature was computed via double differentiation of the B-Spline:

$$\text{radius of curvature} = \frac{1}{\left|\frac{\partial^2 \vec{r}}{\partial s^2}\right|}. \qquad \text{(S6)}$$

The results are shown in Fig. S5. Fig. S5(a) displays contour lengths plotted vs. radii of curvature for reptating 8HTs in networks of different concentration. The curves show a constant contour length irrespective of the radii of curvature. In Fig. S5(b), contour lengths are normalized by the mean $\left\langle l_\mathrm{c}\right\rangle_s$ of the corresponding filament. All curves then collapse onto a master curve, again displaying no trend with curvature. Fig. S5(c) depicts the standard deviation $\sigma\left(l_\mathrm{c}\right)$ plotted vs. $\left\langle l_\mathrm{c}\right\rangle_s$ and illustrates that the deviation is not correlated with the contour length. Both independent measures confirm the inextensible nature of the DNA 8HTs, which is expected to be indicative of other $n$HT species as well.

## V INFLUENCES OF INTERFACIAL ELASTICITY

In literature there is some debate about the influence of interfacial elasticity on bulk elasticity [11]. To

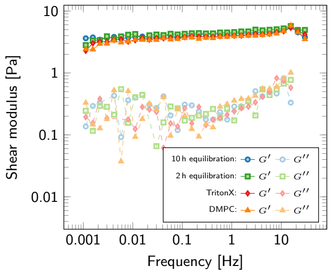


Figure S6. No air-liquid interface effects. We used frequency sweeps ($\gamma = 5\,\%$) of 8HT samples at 8 µM to evaluate the influence of evaporation and gelation effects at the air-water interface. We investigated significantly different equilibration times as well as two methods known to drastically reduce protein clustering at the interface (Triton X and DMPC). All results were consistent showing no indication of drastic influences by evaporation or surface elasticity.

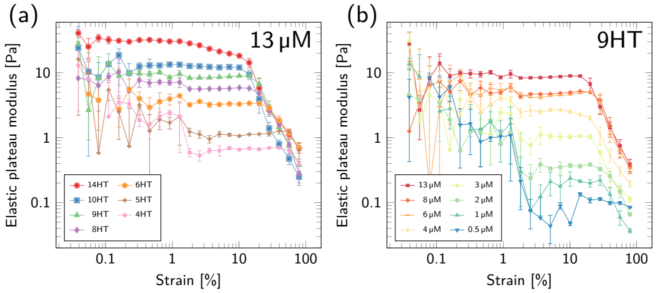


Figure S7. Strain sweeps of $G'(1\,\mathrm{Hz})$. (a) Strain dependence of the elastic plateau modulus for different persistence lengths at 13 µM and (b) for different concentrations with 9HTs.

exclude possible influences of these effects, the surfactant Triton X (at half of the critical micelle concentration) was added to the sample [12] after hybridization. The mixture was equilibrated for two hours before performing measurements. We tested the behavior of the networks with different techniques used to reduce interfacial elasticity. Within the frame of these tests, we compared the surfactant Triton X with the phospholipid DMPC ($0.278\,\mathrm{\mu g\,ml^{-1}}$ pipetted carefully around the sample), which are known to drastically reduce protein clustering at the air-water interface. Additionally, we compared these results to experiments without any passivation agent and examined different equilibration times (two hours and ten hours). All measurements were consistent and yielded results which are within inherent sample-to-sample variations (Fig. S6). Thus, the system is stable under different experimental circumstances and we can conclusively neglect the influence of interfacial elasticity on the presented bulk modulus.

## VI STRAIN SWEEPS: PERSISTENCE LENGTH AND CONCENTRATION

Strain sweeps were performed for all $n$HT types employed in our study and are shown for different persistence length and different concentrations (Fig. S7). For very low strain rates ($< 1\,\%$) the system was prone to noise, especially for less rigid tubes. At moderate strain rates (roughly $3\,\%$ to $10\,\%$) a constant plateau was observed. All measurements presented in the main text were performed within this strain region. For high strain rates ($\sim 15\,\%$ to $20\,\%$) the elastic modulus drastically decreased without showing any strain hardening, which is a characteristic for entangled polymer systems. After high strain rates have been applied to the sample, the elastic modulus did not recover even after several hours (data not shown). We attribute this behavior to irreversible damage caused to the $n$HT network.

## VII SCALING AT DIFFERENT STRAINS OR STRAIN RATES

In the linear elastic regime, the scaling of the plateau modulus $G_0$ is robust and independent of the actual choice of strains and strain rates. We specified $G_0 = G'(1\,\mathrm{Hz}, 5\,\%)$ to facilitate comparison with previous studies [13–15]. Here, the common definition $G_0 = G'(f)|_{G''\to\mathrm{min}}$ [16] was inapplicable due to the pronounced dominance of $G'$ and the resulting masked minimum of $G''$. However, the impact of potential deviations is minute due to the pronounced plateau in $G'$ and the focus on scaling laws rather than absolute values as also described by Hinner et al. [15].

The characteristic scaling of the elastic plateau modulus was found to be $G_0 \propto c^{7/5} l_\mathrm{p}$ for a strain of $5\,\%$ and a strain rate of 1 Hz. This scaling is conserved for a strain of $10\,\%$ or a strain rate of 0.1 Hz (Fig. S8). As demonstrated in section VI, the linear elastic plateau regime extends up to a strain of $10\,\%$ and beyond. Hence, in this regime the scaling is consistent as illustrated in Fig. S8(b) & (e). Complementary, considering the pronounced, flat plateau in the frequency resolved viscoelastic response (cf. Fig. 2(c) and S6) we find the scaling being robust across different strain rates (cf. Fig. S8(c) & (f)).

## VIII END CAPS

Due to the underlying architecture, each of the $n$HT has unpaired single stranded DNA sequences remaining at both ends. To check if these "sticky ends" have a significant effect on the entangled DNA networks, measurements with $n$HTs featuring "blunt ends" were performed. Short DNA strands complementary to unpaired single stranded DNA sequences were added to protect the

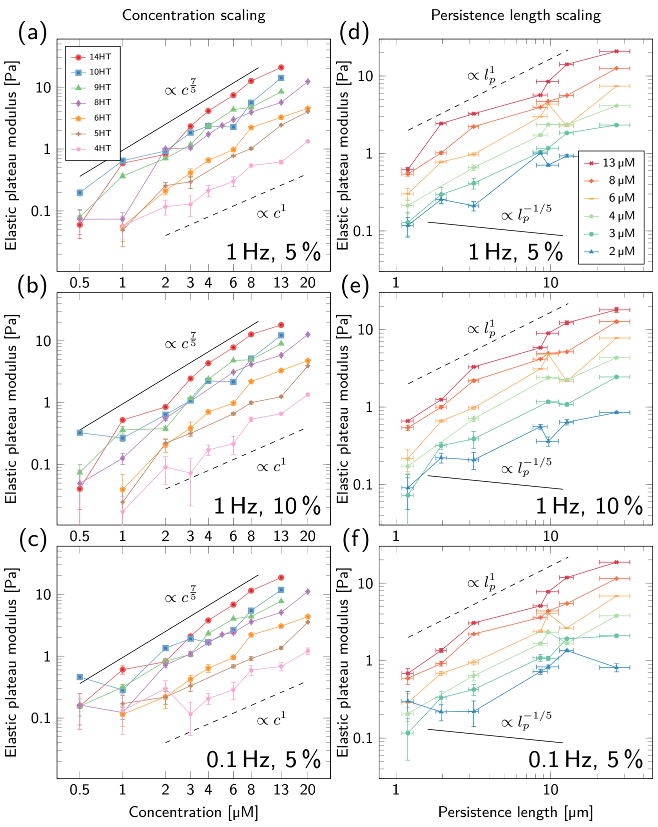


Figure S8. The scaling of the elastic plateau modulus in the linear elastic regime is robust and independent of the actual strain and strain rate. (a) & (d) Scaling of $G_0 = G'(1\,\text{Hz}, 5\,\%)$ as shown in Figure 3. (b) & (e) Scaling of $G'(1\,\text{Hz}, 10\,\%)$ at higher strain. (c) & (f) Scaling of $G'(0.1\,\text{Hz}, 5\,\%)$ at lower strain rate.

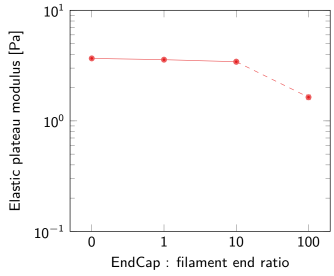


Figure S9. Elastic plateau modulus $G_0$ for 8HT at 8 µM with no end caps, a 1-fold, 10-fold and, 100-fold excess with respect to the calculated $n$HT end concentration.

according end. A simultaneous protection of both ends would lead to a depletion of the capping sequence since complementary motifs are themselves complementary to each other. Thus, we only protected one specific end of the tubes and according capping sequences had only one binding partner in the sample. Using the length distribution and concentrations, we were able to calculate the number of $n$HT ends. To cap potential sticky ends, a mixture of end caps was added in a 1-fold, 10-fold, and 100-fold excess with respect to the calculated $n$HT end concentration (Fig. S9). These end caps were added after the network was already formed. Previous addition of the end caps would have hindered hybridization of the $n$HTs. Samples were equilibrated for eight hours before measurements were performed. For moderate end cap concentrations (1-fold and 10-fold) the network remains unchanged. This strongly indicates that the sticky ends of the $n$HTs have no measurable influence on the network properties. For a 100-fold excess the elastic plateau modulus drops by a factor of two. We address this behavior to a shift in the length distribution of the $n$HTs since such a high concentration of free single stranded DNA also potentially disturbs the preformed $n$HTs through the introduction of internal defects to the tube structure. It is known for other semiflexible filaments that shorter filaments yield softer networks [17]. In the concentration regime addressed in our experiments, the influence of $n$HT ends has been proven to be negligible.


[1] B. Gentry, D. Smith, and J. Käs, Physical Review E **79**, 031916 (2009).
[2] D. Schiffels, T. Liedl, and D. K. Fygenson, ACS Nano **7**, 6700 (2013).
[3] M. B. Smith, H. Li, T. Shen, X. Huang, E. Yusuf, and D. Vavylonis, Cytoskeleton (Hoboken, N.J.) **67**, 693 (2010).
[4] C. Rivetti, M. Guthold, and C. Bustamante, Journal of Molecular Biology **264**, 919 (1996).
[5] N. Mücke, L. Kreplak, R. Kirmse, T. Wedig, H. Herrmann, U. Aebi, and J. Langowski, Journal of Molecular Biology **335**, 1241 (2004).
[6] A. N. Semenov, Journal of the Chemical Society, Faraday Transactions 2: Molecular and Chemical Physics **82**, 317 (1986).
[7] H. Hinsch, J. Wilhelm, and E. Frey, The European Physical Journal E **24**, 35 (2007).
[8] D. Morse, Physical Review E **63**, 031502 (2001).
[9] P. Yin, R. F. Hariadi, S. Sahu, H. M. T. Choi, S. H. Park, T. H. LaBean, and J. H. Reif, Science **321**, 824 (2008).
[10] U. Aebi, R. Millonig, H. Salvo, and A. Engel, Annals of the New York Academy of Sciences **483**, 100 (1986).
[11] S. Yamada, D. Wirtz, and P. A. Coulombe, Journal of Structural Biology **143**, 45 (2003).
[12] O. Mueller, H. E. Gaub, M. Baermann, and E. Sackmann, Macromolecules **24**, 3111 (1991).
[13] M. Tassieri, R. Evans, L. Barbu-Tudoran, G. Khaname, J. Trinick, and T. Waigh, Physical Review Letters **101**, 198301 (2008).
[14] A. Palmer, T. G. Mason, J. Xu, S. C. Kuo, and D. Wirtz, Biophysical Journal **76**, 1063 (1999).
[15] B. Hinner, M. Tempel, E. Sackmann, K. Kroy, and E. Frey, Physical Review Letters **81**, 2614 (1998).
[16] C. Liu, J. He, E. v. Ruymbeke, R. Keunings, and C. Bailly, Polymer **47**, 4461 (2006).
[17] F. G. Schmidt, B. Hinner, and E. Sackmann, Physical Review E **61**, 5646 (2000).
